# Supplementary material for: Nerfies: Deformable Neural Radiance Fields
Source: arXiv:2011.12948 source file (2021-09-10)
Supplement: Supplementary file 1 [file A0_supplementary.tex]

\documentclass[10pt,twocolumn,letterpaper]{article}

\usepackage{iccv}
\usepackage{times}
\usepackage{epsfig}
\usepackage{graphicx}
\usepackage{amsmath}
\usepackage{amssymb}

\usepackage{subcaption}
\usepackage{commath}
\usepackage{booktabs}
\usepackage[numbers,sort]{natbib}
\usepackage{siunitx}
\usepackage{bold-extra}
\usepackage[T1]{fontenc}
\usepackage{contour}% http://ctan.org/pkg/contour
\usepackage{microtype}      % microtypography
\usepackage{booktabs}       % professional-quality tables
\usepackage{multirow}
\usepackage{multicol}
\usepackage{tabu}
\usepackage[symbol]{footmisc}
\usepackage{xr-hyper}

% Cross-referencing.
\makeatletter
\newcommand*{\addFileDependency}[1]{% argument=file name and extension
  \typeout{(#1)}
  \@addtofilelist{#1}
  \IfFileExists{#1}{}{\typeout{No file #1.}}
}
\makeatother

\newcommand*{\myexternaldocument}[1]{%
    \externaldocument{#1}%
    \addFileDependency{#1.tex}%
    \addFileDependency{#1.aux}%
}

\myexternaldocument{00_main.tex}

\newif\ifdraft
\drafttrue

% Include other packages here, before hyperref.

% If you comment hyperref and then uncomment it, you should delete
% egpaper.aux before re-running latex.  (Or just hit 'q' on the first latex
% run, let it finish, and you should be clear).
\usepackage[pagebackref=true,breaklinks=true,colorlinks,bookmarks=false]{hyperref}

\iccvfinalcopy % *** Uncomment this line for the final submission

 % *** Enter the ICCV Paper ID here

% Pages are numbered in submission mode, and unnumbered in camera-ready
\ificcvfinal\pagestyle{empty}\fi

\input{commands.tex}

\begin{document}

%%%%%%%%% TITLE
\title{Nerfies: Deformable Neural Radiance Fields\\(Supplementary Materials)}

\author{
Keunhong Park\textsuperscript{1}\footnotemark
\and Utkarsh Sinha\textsuperscript{2}
\and Jonathan T. Barron\textsuperscript{2}
\and Sofien Bouaziz\textsuperscript{2}
\and Dan B Goldman\textsuperscript{2}
\and Steven M. Seitz\textsuperscript{1,2}
\and Ricardo Martin-Brualla\textsuperscript{2} \smallskip
\and
\textsuperscript{1}University of Washington\qquad 
\textsuperscript{2}Google Research \\ \rurl{nerfies.github.io}
}

\twocolumn[{
\renewcommand\twocolumn[1][]{#1}
\maketitle
}]

%%%%%%%%% ABSTRACT
\input{A1_appendix}

% Hack
\clearpage

{\small
\bibliographystyle{ieee_fullname}
\bibliography{00_main}
}

\end{document}
